# Supplementary material for: OntoMerger: An Ontology Integration Library for Deduplicating and Connecting Knowledge Graph Nodes
Source: arXiv:2206.02238 source file (2022-06-05)
Supplement: Supplementary file 1 [file appendix.tex]

\appendix

\section{Multi-scale node representations}
